# Supplementary material for: Fawkes: Protecting Privacy against Unauthorized Deep Learning Models
Source: arXiv:2002.08327 source file (2020-06-23)
Supplement: Supplementary file 1 [file appendix.tex]

\section{Appendix}
\label{sec:appendix}

\begin{figure}[t]
  \centering
  \begin{minipage}{0.32\textwidth}
    \centering
    \includegraphics[width=1\textwidth]{plots/eval/pubfig_same_teacher_nclass.eps}
    \vspace{-0.1in}
    \caption{Protection performance as number of labels sampled for training in
      \pubfig{} dataset increases (results averaged over 10 runs).}
    \label{fig:scrub_density}
  \end{minipage}
\end{figure}
